# Supplementary material for: Zero-Threshold PT-Symmetric Polariton-Raman Laser
Source: arXiv:2305.17475 ancillary file (2025-02-01)
Supplement: Supplementary file 1 [file supplemental_material.pdf]

# Supplemental Material

# Zero-Threshold PT-Symmetric Polariton-Raman Laser

Avijit Dhara[1†], Pritam Das[1†], Devarshi Chakrabarty[1†], Kritika Ghosh[2], Ayan Roy Chaudhuri[2], Sajal Dhara[1*]

[1]*Department of Physics, IIT Kharagpur, Kharagpur-721302, India*

[2]*Materials Science Centre, IIT Kharagpur, Kharagpur-721302, India*

[†] *These authors contributed equally*

[*] *Corresponding author. email: sajaldhara@phy.iitkgp.ac.in*

## List of Contents:

**Notes S1-S4**

**Figs. S1-S10**

**References**

## Note S1. Methods

### Sample fabrication

We prepared three samples of $ReS_2$ with the same thickness: two embedded in a microcavity and the other stacked on $SiO_2$/Si (referred to as a 'bare' sample). The microcavity consists of two distributed Bragg reflectors (DBRs). The bottom mirror comprises 10 pairs of $SiO_2/Ta_2O_5$ films, grown using the RF sputtering technique. Two $ReS_2$ crystal of thickness ~10 nm are exfoliated by the dry transfer method and transferred on the bottom mirror. The top DBR of 8 pairs of $SiO_2/Ta_2O_5$ is then deposited using the same sputtering method. The other sample is prepared by dry transfer of exfoliated 10 nm thick $ReS_2$ crystal on the Si/$SiO_2$ substrate. We estimate the sample thickness from optical contrast. Sample image is shown in Fig. S1.

### Measurement

All optical measurements were performed with the sample placed in a closed cycle microscopy cryostat (Montana Instruments) with a variable temperature range of 3.2 to 295 K. For the Raman study, we excite the sample using backscattering geometry with a Ti: Sapphire laser (Coherent—MIRA) in CW mode with a pump energy of 1.564 eV ($\lambda_{excitation} = 792.8$ nm). The excitation path contains a linear polarizer followed by a half-wave plate mounted on a motorized rotational stage to control the polarization of the pump beam. Polarization state of light beam was preserved throughout the optical path via a special design in our optical setup as discussed elsewhere [1] for polarization resolved Raman spectroscopy. The laser beam was focused to a spot size ∼1 µm by a 60X objective lens with numerical aperture of 0.7. The Raman stokes signal is collected through the same objective lens and dispersed by a diffraction grating with 1200 grooves per mm and detected by a nitrogen-cooled CCD (Pylon 400) with spectral resolution of 0.5 $cm^{-1}$. In the temperature dependent power variation study, to attenuate scattered light of the laser from the optical elements in the beam path and increase the signal-to-noise ratio, an analyzer is kept before the spectrometer, crossed with the laser polarization. A broadband light source (Thorlabs SLS202L) is used for reflectance measurements.

**Anisotropic polariton dispersion and cavity parameters**

A detailed study of exciton-polariton dispersions in this system has been presented in a our recent work [2]. The maximum value of the coupling strengths at two different polarizations of the probe beam are estimated to be 14.5 and 18.6 meV respectively at 4 K. The coupling strengths can be tuned by rotating the pump polarization, and the system can be tuned from the strong to weak coupling regime. The Q factor for the composite cavity consisting of $SiO_2$ and $ReS_2$ is ~300.

**Second order correlation measurements**

To measure the $g^{(2)}$ correlation of the Raman emission from the microcavity, we have used single photon detectors from IDQ, with a timing resolution (FWHM) of 40 ps, and TCSPC module of time resolution 2 ps from Becker & Hickl (SPC-130IN). We filtered out the specific Raman signal using a monochromator with spectral resolution of 0.9 Å. After carefully aligning our HBT interferometer, we characterized the $g^{(2)}$ of the pump obtained in pulsed (ps) and CW mode from our tunable Ti-Sapphire laser reflected from the microcavity, as shown in Fig. S10. In pulsed mode, there is a separation of 13.2 ns between the pulses, which matches well with the repetition rate of the laser which is 76 MHz.

The variation in $g^{(2)}(\tau)\, for$ the pump laser is modelled as follows. For a given amplitude $\mathrm{E} = \mathrm{E_0 cos\omega_0 t} + \mathrm{E_1}[\cos(\overline{\omega_0 + \Delta\omega} \mathrm{t}) + \cos(\overline{\omega_0 - \Delta\omega}\mathrm{t})]$, we can evaluate $g^{(2)}(\tau)$ as $\mathrm{A} + B\cos(2\Delta\omega\tau) + C\cos(\omega_0\tau)$. Due to the finite time resolution (40 ps) of the photodetectors, the term $C\cos(\omega_0\tau)$ with corresponding time period ~3 attoseconds has no contribution to the experimental observation. Thus, we only observe $g^{(2)}(\tau) = \mathrm{A} + B\cos(2\Delta\omega\tau)$. Fourier transform of the of the $g^{(2)}(\tau)$ shows a similar value of the $\Delta\omega$ (using Siegert relation) obtained from the above analysis.

Due to the limited strength of the Raman signal reaching the photodetector (corresponding to a count rate of 13,000 photons/second), we had chosen a bin size of 96 ps in order to build reasonable statistics over 32 hours.

## Note S2. Stacking order in $ReS_2$

We identify several Raman modes as shown in Fig. S2, which exactly match with existing literature. A list of the observed Raman modes with their symmetry and labeling notation is presented in Table S2.

Recently, it has been reported that $ReS_2$ crystal has two stable stacking orders (AA and AB) [3], which have been identified by the separation between the $A_g^4$ and $A_g^1$ modes. The separation between these two modes in both cases (inside microcavity and bare sample) is 13 $\mathrm{cm}^{-1}$, as found in AA stacking $ReS_2$ crystal, as shown in Fig. S3.

## Note S3. Microscopic theory for stimulated Raman scattering in anisotropic microcavity

To derive the microscopic model for Raman scattering, we consider the vibrational states of the ground electronic state of $ReS_2$. We use a two-dimensional model, in which the potential landscape of this state can be approximated as a displaced harmonic potential. The induced polarization density of $ReS_2$ can be written as [4]:

$$P_j = \varepsilon_0 \chi_{jk} E_k = \varepsilon_0 \left( \left(\chi_{jk}\right)_0 + \left(\frac{\partial \chi_{jk}}{\partial q_1}\right)_0 q_1 + \left(\frac{\partial \chi_{jk}}{\partial q_2}\right)_0 q_2 \right) E_k \qquad (2)$$

Here, $q_1$, $q_2$ are the two normal coordinates of vibration associated with the two polarized Stokes emissions. $\left(\chi_{jk}\right)_0$ is the susceptibility tensor element in the equilibrium position. $E_k$ is the electric field component.

Therefore, from (2) the interaction Hamiltonian density contributing to the Raman process can be expressed as follows:

$$H_{int} = -\sum_{j=1}^{2} P_j E_j = -\sum_{j=1}^{2} \sum_{k=1}^{2} \varepsilon_0 \left( \left( \frac{\partial \chi_{jk}}{\partial q_1} \right)_0 q_1 + \left( \frac{\partial \chi_{jk}}{\partial q_2} \right)_0 q_2 \right) E_k E_j$$

$$= -\sum_{j=1}^{2} \sum_{k=1}^{2} \sum_{\mu=1}^{2} \varepsilon_0 R_{jk\mu}\, q_\mu E_k E_j \text{ …….. (3)}$$

Where $R_{jk\mu} = \left( \frac{\partial \chi_{jk}}{\partial q_\mu} \right)$ is the Raman tensor element. To capture the effect of stimulated Raman scattering, we consider the system has been excited in the presence of both pump and Stokes frequencies with $d_1$ and $d_2$ polarization. i.e.

$$E_j(t) = E_{lj} \cos \omega_l t + E_{sj} \cos \omega_s t$$

Where $j = 1$ and 2 indicate $d_1$ and $d_2$ polarizations of the electric field.

Quantized electric fields inside microcavity can be expressed using creation and annihilation operators corresponding to the pump and Stokes photons, denoted as$(a_{lj}^{+}, a_{lj})$ and $(a_{sj}^{+}, a_{sj})$. Here, the index $j$ indicates the polarization mode, as mentioned previously.

The operator $\widehat{E_j}$ can be expressed in terms of the photon creation and annihilation operators:

$$\widehat{E_j} = \hat{E}_{lj} + \hat{E}_{sj} = \left[ i\sqrt{\frac{\hbar\omega_l}{2\varepsilon_0 V_{eff}}}\,(a_{lj}^{+} - a_{lj}) + i\sqrt{\frac{\hbar\omega_s}{2\varepsilon_0 V_{eff}}}\,(a_{sj}^{+} - a_{sj}) \right]$$

In the harmonic potential approximation, the vibrational levels separated by phonon frequency $\nu$ can be quantized using the phonon creation and annihilation operators $b_j^{+}$and $b_j$. We can now define the normal coordinate as $\hat{q}_j = q_0(b_j^{+} + b_j)$where, $q_0$ is zero-point amplitude of vibration. Here, the index $j = 1$ and 2 indicate normal coordinate of vibration in two orthogonal directions.

The Hamiltonian density of the system can be written as,

$$H = H_0 + H_{int}$$

Where, $H_0$ is the unperturbed Hamiltonian density:

$$H_0 = \sum_{j=1}^{2} \left[ \hbar\omega_l \left( a_{lj}^{+} a_{lj} + \frac{1}{2} \right) + \hbar\omega_s \left( a_{sj}^{+} a_{sj} + \frac{1}{2} \right) + \hbar\nu \left( b_j^{+} b_j + \frac{1}{2} \right) \right]$$

The interaction Hamiltonian density given in Eqn. (3) can be written as:

$$H_{int} = -\sum_{j=1}^{2} \sum_{k=1}^{2} \sum_{\mu=1}^{2} [\varepsilon_0 R_{jk\mu} \hat{q}_\mu \hat{E}_j \hat{E}_k]$$

We consider the non-zero contributions of the Raman processes involving emission and absorption of polarized Stokes photons due to interaction with co-polarized and cross-polarized pump photons are denoted by $H_{int}^{co}$ and $H_{int}^{cross}$ respectively. These processes are illustrated in Fig. S8.

Therefore, the interaction Hamiltonian density is reduced to $H_{int} = H_{int}^{co} + H_{int}^{cross}$, where:

$$H_{int}^{co} = -\sum_{j=1}^{2} [\varepsilon_0 R_{jjj} \hat{q}_j \hat{E}_{lj} \hat{E}_{sj}]$$

$$H_{int}^{cross} = -\sum_{j=1}^{2} \sum_{\{j \neq k, k=1\}}^{2} [\varepsilon_0 R_{jkk} \hat{q}_k \hat{E}_{lj} \hat{E}_{sk}]$$

After substituting the expression of $\hat{E}_{lj}$, $\hat{E}_{sj}$, and $\hat{Q}_j$, the non-zero terms contributing to the Raman processes can be written as:

$H_{int}^{co} = -\hbar\Omega \sum_{j=1}^{2} R_{jjj}\left[\left(a_{lj}a_{sj}^{+}b_j^{+}\right) + (h.c)\right]$ , and $H_{int}^{cross} = -\hbar\Omega \sum_{j=1}^{2} \sum_{\{j\neq k,k=1\}}^{2} R_{jkk}\left[\left(a_{lj}a_{sk}^{+}b_k^{+}\right) + (h.c)\right]$

Where $\Omega = \frac{q_0\sqrt{\omega_s\omega_l}}{V_{eff}}$. The composite state of the system is constructed from the tensor product of the pump, Stokes photons, and phonon number states, represented as$|\, n_{l1}, n_{l2}, n_{s1}, n_{s2}, n_1, n_2\rangle$. Here, $n_{lj}, n_{sj}, n_j$ denote the photon numbers of the pump, Stokes modes and phonon number respectively, with index $j$ = 1,2 implying $d_1$, $d_2$ polarization of photons and excited phonon modes corresponding to two polarized Stokes emissions.

We use Bose-Einstein statistics for phonon occupation number in ground and 1st excited state of vibrational energy level denoted as $P_a$ and $P_b$ respectively. The transition rate for emission of $j^{th}$-Stokes photons via annihilation of co and cross polarized pump photons are denoted by $\Gamma_{jj}$ and $\Gamma_{kj}$ respectively.

Consequently, Total emission rate for $j^{th}$-Stokes photons:

$$\Gamma = \Gamma_{jj} + \Gamma_{kj}$$

$$\Gamma_{jj} = \frac{2\pi}{\hbar^2} V_{eff}^2\, P_a \left|\langle n_{lj} - 1, n_{sj} + 1, n_{lk}, n_{sk}, \delta_{1j}, \delta_{2j} \mid \hbar\Omega R_{jjj}\left(a_{lj}a_{sj}^{+}b_j^{+}\right)\right| n_{lj}, n_{sj}, n_{lk}, n_{sk}, 0,0\rangle\Big|^2 \rho_c(\omega_s)$$

$$=\left[\frac{2\pi}{\hbar^2}\left(\hbar\Omega V_{eff}\right)^2 \rho_0\right] R_{jjj} P_a n_{lj}\left(n_{sj} + 1\right) F_j$$

$$= \alpha_{jj} P_a n_{lj}\left(n_{sj} + 1\right) F_j$$

$$\Gamma_{kj} = \frac{2\pi}{\hbar^2} V_{eff}^2 P_a \left|\langle n_{lj}, n_{sj,} + 1, n_{lk} - 1, n_{sk}, \delta_{2j}, \delta_{1j} \right| \hbar\Omega R_{kjj}\left(a_{lk}a_{sj}^{+}b_j^{+}\right)\Big| n_{lj}, n_{sj}, n_{lk}, n_{sk}, 0,0\rangle\Big|^2 \rho_c(\omega_s)$$

$$= \left[\frac{2\pi}{\hbar^2}\left(\hbar\Omega V_{eff}\right)^2 \rho_0\right] R_{kj}\ P_a n_{lk}\left(n_{sj} + 1\right) F_j$$

$$= \alpha_{kj} P_a n_{lk}\left(n_{sj} + 1\right) F_j$$

Here, $\delta_{1j}, \delta_{2j}$ are the Kronecker delta and $\alpha_{kj} = R_{kjj}\left[\frac{2\pi}{\hbar^2}\left(\hbar\Omega V_{eff}\right)^2 \rho_0\right]$ is Raman tensor element of bulk $ReS_2$ multiplied with a constant. $F_j$ is the Purcell factor corresponding to the $d_j$-polarized polariton mode by which the vacuum photon density $\rho_0(\omega_s)$ is enhanced inside the microcavity [5].

Similarly, the rates of the inverse processes, where a pump photon is emitted while a co-polarized and cross polarized Stokes photon is absorbed, can be written,

$$\Gamma' = \Gamma'_{jj} + \Gamma'_{kj} = \alpha_{jj} P_b n_{sj}\left(n_{lj} + 1\right) F_j + \alpha_{kj} P_b n_{sj}(n_{lk} + 1) F_j$$

Therefore, the overall rate of change of the $j^{th}$-Stokes photons number can be written as:

$$\frac{dn_{sj}}{dt} = \Gamma - \Gamma' - \frac{n_{sj}}{\tau_j}$$

$$= \left[\alpha_{jj} F_j (P_a - P_b) n_{lj} + \alpha_{kj} F_j (P_a - P_b) n_{lk} - P_b F_j (\alpha_{jj} + \alpha_{kj}) - \frac{1}{\tau_j}\right] n_{sj} + P_a F_j (\alpha_{jj} n_{lj} + \alpha_{kj} n_{lk})$$

Where $\tau_j$ is the finite lifetime of Stokes photon due cavity loss. We write $\alpha_{kj}(P_a - P_b) = g_{kj}$, where $g_{kj}$ is the stimulated Raman gain per unit intensity, and $F_i$ is the Purcell factor corresponding to the $d_i$-polarized polariton mode by which the Raman gain is enhanced inside the microcavity.

The pump photon number ($n_{lj}$) can be controlled with a polarizer as a function of polarizer angle $\theta$, with respect to the lab frame which can be written as follows:

$$n_{lj} = Q_j I_0 \text{Cos}(\phi_j - \theta)^2$$

Where $I_0$ is the intensity of pump photons inside the cavity, $Q_j$ being the quality factor of the cavity mode resonant with the pump frequency. Here, $\phi_{j=1,2}$ is the angle of $d_{j=1,2}$ axis of the sample in the lab-frame. Thus,

$$\frac{dn_{sj}}{dt} = [F_j\{g_{jj}Q_j I_0 Cos(\phi_j - \theta)^2 + g_{kj}Q_k I_0 Cos(\phi_k - \theta)^2 - (g_{jj} + g_{kj})f(T)\} - \frac{1}{\tau_j}]n_{sj} + F_j(f(T) + 1)\left[\left(g_{jj}Q_j I_0 Cos(\phi_j - \theta)^2 + g_{kj}Q_k I_0 Cos(\phi_k - \theta)^2\right)\right]$$

Where $f(T) = \frac{1-\exp\left(-\frac{\hbar\omega}{2k}\right)}{\exp\left(\frac{\hbar\omega}{kT}\right)-1}$. We define $\xi_j$ and $c_j$:

$$\xi_j = F_j[g_{jj}Q_j I_0 \text{Cos}(\phi_j - \theta)^2 + g_{kj}Q_k I_0 \text{Cos}(\phi_k - \theta)^2 - (g_{jj} + g_{jk})f(T)]$$

$$c_j = F_j(f(T) + 1)\left[\left(g_{jj}Q_j I_0 Cos(\phi_j - \theta)^2 + g_{kj}Q_k I_0 Cos(\phi_k - \theta)^2\right)\right]$$

Such that, the rate equation can be written as:

$$\frac{dn_{sj}}{dt} = \left[\xi_j - \frac{1}{\tau_j}\right]n_{sj} + c_j \text{.................................}(4)$$

We identify the coefficient $\xi_j$ as the gain coefficient for the j[th] Stokes modes. Due to the loss in the cavity, the overall coefficient $\left(\xi_j - \frac{1}{\tau_j}\right)$ of $n_{sj}$ becomes negative which enables the system to reach the steady state. For steady-state condition, $\frac{dn_{sj}}{dt} = 0$. Thus, solving for the steady-state value of $n_{si}$, we get:

$$n_{sj} = -\frac{c_j}{\xi_j - \frac{1}{\tau_j}}$$

Considering a collection efficiency $c'$, the Stokes emission intensity can thus be written as:

$$I_{out,j} = \frac{c' n_{sj}}{\tau_j}$$

This model is used to fit the intensity data shown in Fig. 3. We obtain the ratios among the four Raman gain tensor elements. The experimental constants and parameter values obtained from fitting are given in Table S1.

## Note S3(b). Power dependence and $\beta$ factor of zero threshold Raman laser

To explain the observed linear power dependence (shown in Fig. 2(b)), of the zero-threshold laser for $d_1$ polarized pump with pump photon number $n_l = n_{l1}$, we take the approximation $n_{l2} \sim 0$ and consider the rate equation of the co-polarized Stokes mode ($n_s = n_{s1}$), which experiences much greater gain ( $\xi_1 \gg \xi_2$).

By taking a large photon number approximation in the beginning of the microscopic model it can be shown that above equation (4) can have an alternative and simplified form:

$$\frac{dn_s}{dt} = [\beta F_1 g_{11} n_l - \frac{1}{\tau_1}]n_s$$

Where, a factor $\beta$ is introduced in the $1^{st}$ term at the right-hand side to take into account the spectral overlap [6–11] of the Raman and the cavity mode.

Also, the time evolution of the pump photon number $n_l$ can be written as,

$$\frac{dn_l}{dt} = P_{in} - \beta F_1 g_{11} n_l n_s - (1-\beta)\gamma n_l$$

Here, $P_{in}, \gamma$ is the generation rate and the scattering rate from pump photon to the cross-polarized Stokes modes, or other radiative and non-radiative processes.
By finding the steady-state solutions of the above system of equations, we find the output intensity is directly proportional to $P_{in}$, for $\beta$=1:

$$I_{out} = \frac{c' n_s}{\tau} \propto cP_{in}$$

## Note S4. Comparison between Conventional laser and Polariton Raman Laser

In a conventional laser, multiple cavity modes exist within a single emission profile in the frequency domain, i.e., different frequencies cavity modes linewidth $\Delta\omega_c$ is much narrower than the emission linewidth (gain profile linewidth) $\Delta\omega$ as shown on the left in Fig. S9. Consequently, there is competition among different cavity modes for pump photons. Therefore, by definition, for multimode lasing, spontaneous emission coupling ($\beta$) factor for each cavity modes become less than unity.

$$\beta_i = \frac{\int C_i(\omega - \omega_i)E(\omega)d\omega}{\sum_j \int C_j(\omega - \omega_j)E(\omega)d\omega}$$

However, in our case, polariton modes function as cavity modes, while the Raman modes' profile operates as an emission profile. Thus, we find ourselves in the opposite limit of the conventional laser case. Specifically, the emission linewidth (individual Raman modes) ($\Delta\hbar\omega\sim$ 0.1 meV) is much narrower than the cavity modes' linewidth ($\Delta\hbar\omega_c\sim$ 22 meV) (shown on the right in Fig. S9). Since each Raman modes is overlap with not only one cavity mode (the lower polariton branch of X1) in frequency domain, but also the TE-TM degeneracy is lifted due to anisotropy. Consequently, it becomes a single mode laser for individual Raman frequencies which shows up as zero-threshold laser in the PT-symmetric condition with $\beta_i$ = 1. The system can also be viewed as a collection of single mode lasers at different frequencies. This is the rationale used to treat the individual Raman modes separately in our rate equation model.

However, when we observe finite threshold in the PT-symmetry broken phase, the emission consists of two polarization states at same frequency. Hence it is no more a single-mode laser, with $\beta_i$ < 1.

**Table S1: Parameter values obtained from fitting pump dependence at 4K and room temperature**

<u>Experimental constants (temperature independent):</u>

$\lambda$ ($A_g^{12}$) = 0.8128 $\mu m$, $L_{SiO2}$ = 250 nm, $L_{ReS2}$ = 10 nm, n = $\frac{n_{SiO}\ L_{SiO2} + n_{ReS2} L_{ReS2}}{L_{SiO2}+L_{ReS2}}$ = 1.88,
$V_{eff}$ = Sample area × $L_{ReS2}$ = 0.01 $\mu m^3$.

Formulae used:

$$\tau = \frac{Q}{\omega_s} \frac{(\Delta\omega_c)^2}{4(\omega_s-\omega_c)^2+(\Delta\omega_c)^2}\ ;\ F = \frac{3Q\left(\frac{\lambda}{n}\right)^3}{4\pi^2 V_{eff}} \times \frac{(\Delta\omega_c)^2}{4(\omega_s-\omega_c)^2+(\Delta\omega_c)^2}\ ;$$

Cavity parameters obtained from angle resolved reflectivity data (temperature dependent):

| Temp | $\Delta\omega_c$ $(meV)$ | $\omega_{c1}$ $(eV)$ | $\omega_{c2}$ $(eV)$ | $\omega_s$ $(eV)$ | $Q_1$ | $Q_2$ | $\tau_1$ (ps) | $\tau_2$ (ps) | $F_1$ | $F_2$ |
|---|---|---|---|---|---|---|---|---|---|---|
| 10K | 10 | 1.530 | 1.564 | 1.526 | 153.0 | 156.4 | 0.23 | 0.007 | 53.1 | 1.6 |
| 300K | 20 | 1.548 | 1.548 | 1.538 | 77.4 | 78.1 | 0.10 | 0.031 | 7.9 | 3.4 |

Raman gain tensor ratios obtained from the fitting of experimental data with theory:

| Temp | $\frac{g_{22}}{g_{11}}$ | $\frac{g_{12}}{g_{11}}$ | $\frac{g_{21}}{g_{11}}$ |
|---|---|---|---|
| 10K | 2.52 | 0.22 | 0.43 |
| 300K | 1.67 | 0.40 | 0.23 |

**Table S2: List of 17 observed Raman modes with labelling scheme**

| **Raman Frequency ($cm^{-1}$)** | **Symmetry** | **Labelling scheme** |
|---|---|---|
| 139 | $A_g$ − like | $A_g^4$ |
| 144 | $A_g$ − like | $A_g^5$ |
| 152 | $E_g$ − like | $A_g^1$ |
| 162 | $E_g$ − like | $A_g^6$ |
| 214 | $E_g$ − like | $A_g^7$ |
| 236 | $E_g$ − like | $A_g^8$ |
| 276 | $C_p$ | $A_g^9$ |
| 284 | $C_p$ | $A_g^{10}$ |
| 311 | $E_g$ − like | $A_g^{12}$ |
| 320 | $C_p$ | $A_g^{13}$ |
| 325 | $C_p$ | $A_g^{14}$ |
| 349 | $C_p$ | $A_g^{15}$ |
| 369 | $C_p$ | $A_g^{16}$ |
| 378 | $C_p$ | $A_g^{17}$ |
| 408 | $C_p$ | $A_g^{18}$ |
| 420 | $A_g$ − like | $A_g^3$ |
| 440 | $A_g$ − like | $A_g^2$ |

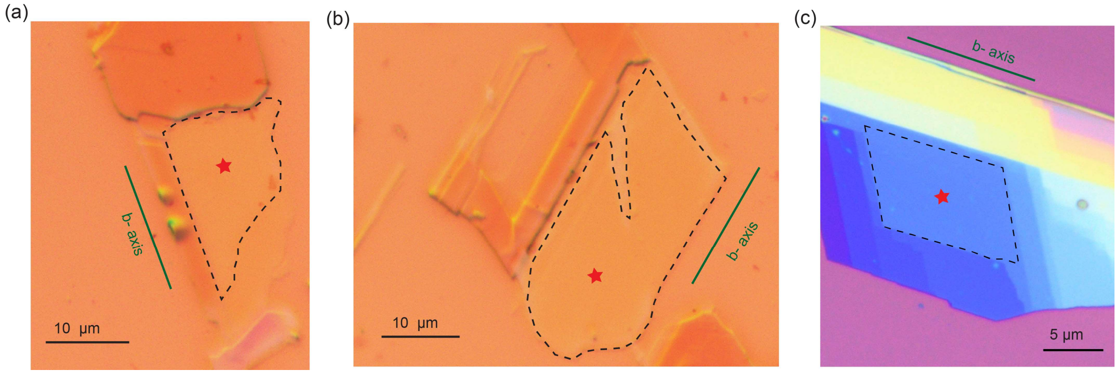


**Fig. S1 | Optical microscope images of** (a) $ReS_2$ inside microcavity. All data presented in Figs.1-5 in the article correspond to experiments done on this sample. (b) Different $ReS_2$ samples inside microcavity with same thickness as (a) whose corresponding experimental data is shown in Fig. S8. (c) Bare $ReS_2$ ($ReS_2$ on $SiO_2$/Si). The black dotted lines indicate the boundary of the sample section that is 10 nm in thickness. The red starting point denotes the excitation point.

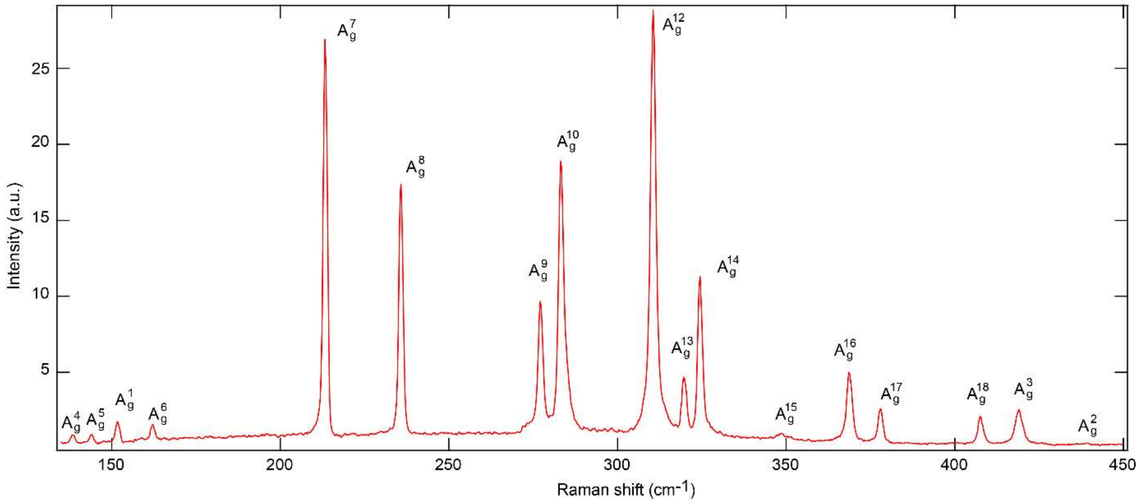


**Fig. S2 |** Raman spectra measured for $ReS_2$ inside microcavity, with the distinct modes labelled.

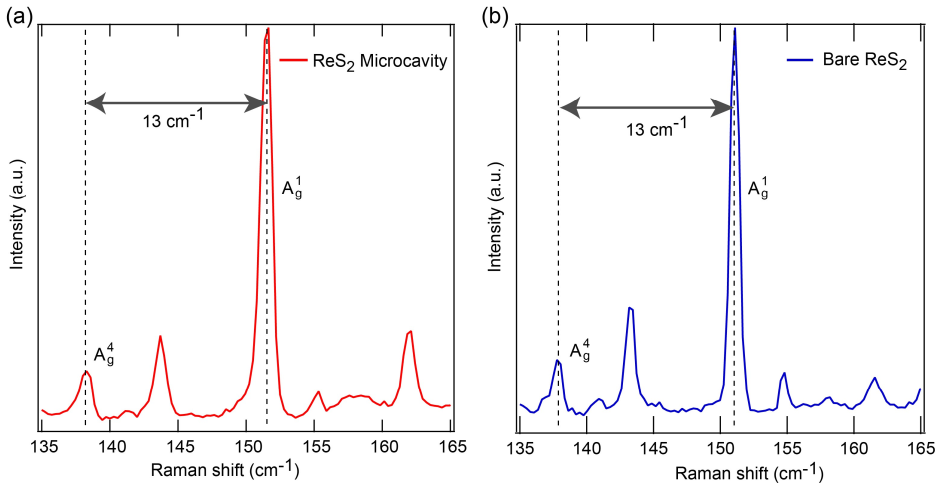


**Fig. S3 | Stacking order dependent Raman modes in $ReS_2$.** The $A_g^4$ and $A_g^1$ Raman modes exhibit a separation of 13 cm$^{-1}$ indicating AA stacking in both scenarios: (**a**) $ReS_2$ within the microcavity and (**b**) $ReS_2$ on $SiO_2$/Si

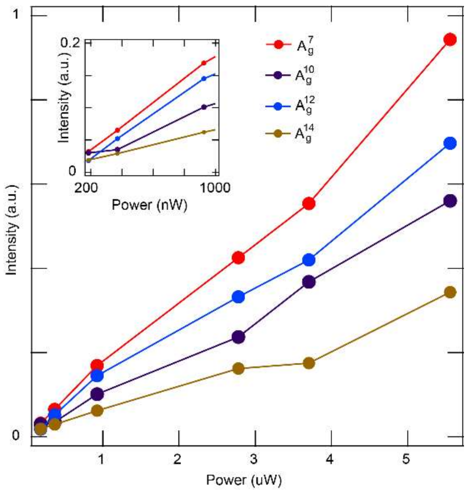


**Fig. S4** | Power dependence of Raman intensity at low power regime.

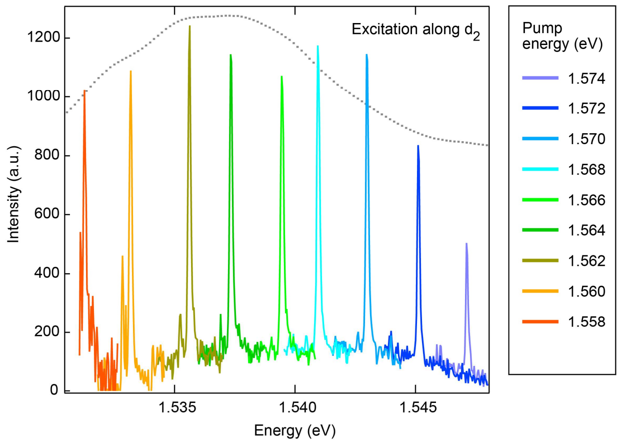


**Fig. S5** | Intensity variation of the $A_g^7$ mode spectrum for $d_2$-polarized pump, with different colors representing different pump energies. The reflectance line plot for $d_2$ polarization from Fig 1(c) has been inverted and overlaid as a visual aid.

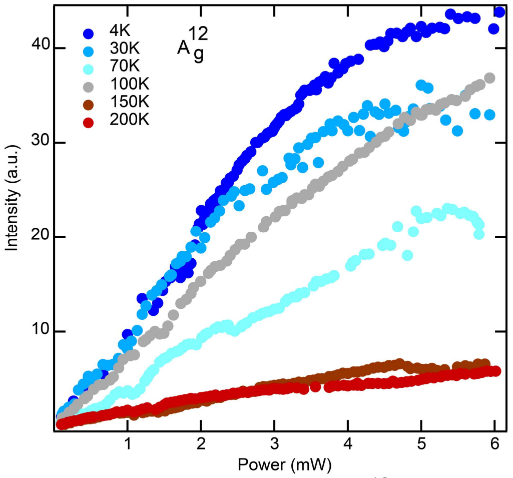


**Fig. S6 |** Evolution of power dependence with temperature for $A_g^{12}$ mode, with $d_1$ polarized pump.

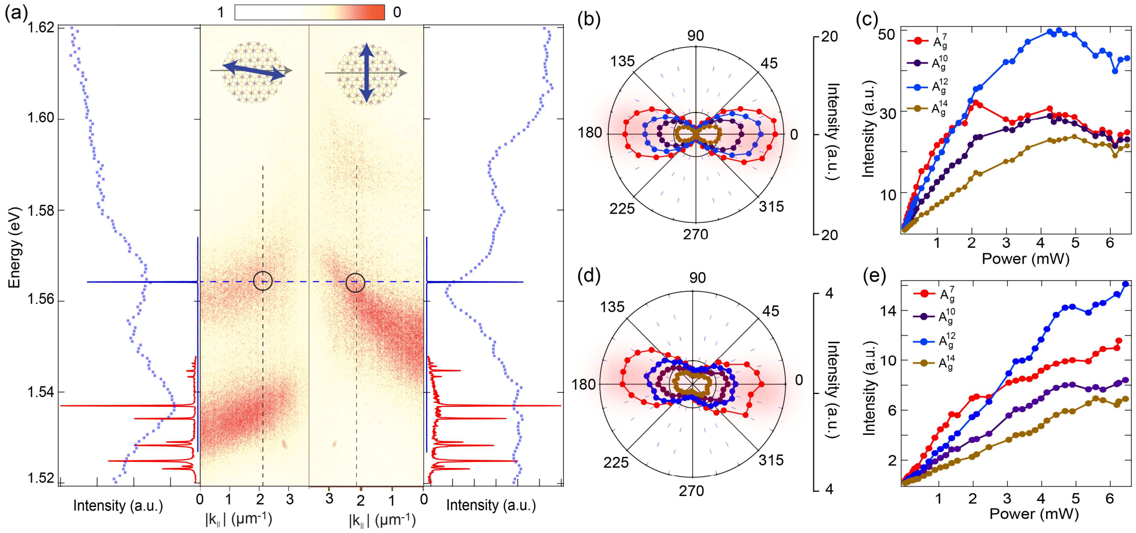


**Fig. S7 | Experimental results for alternative sample shown in Fig. S1.** (a) Angle resolved reflectance for probe beam polarization along $d_1$ (right) and $d_2$ (left) axis. Black circles mark the $k_{||}$ values where the pump energy coincides with the polariton bands. Adjacent plots along the extreme left and extreme right show corresponding line profile at these $k_{||}$ values and the Raman spectrum (red) when the pump beam (blue) is polarized along those directions. (b) Polar plot of emission intensity as a function of analyser angle for the pump beam polarization along $d_1$, showing a strongly polarized emission. (c) Power dependence data for excitation along $d_1$ showing linear dependence followed by saturation at higher power. (d), (e). Same as (b), (c) for $d_2$ polarized pump.

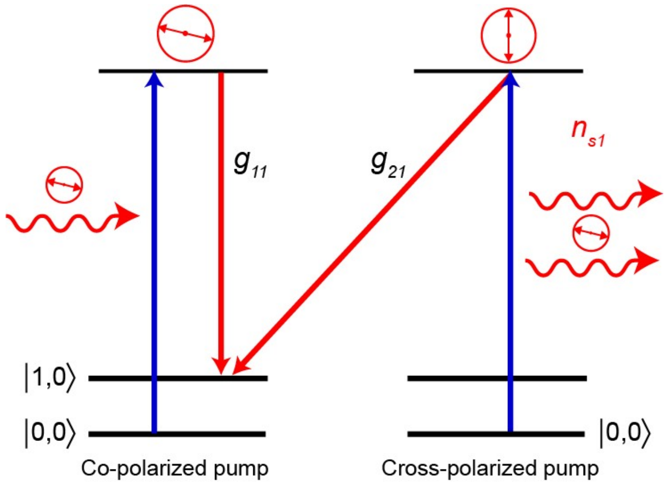


**Fig. S8 | Schematic of the stimulated Raman scattering processes.** Two possible scattering mechanisms for generation of one of the polarized Stokes modes by co-polarized and cross polarized pump considered in the microscopic model.

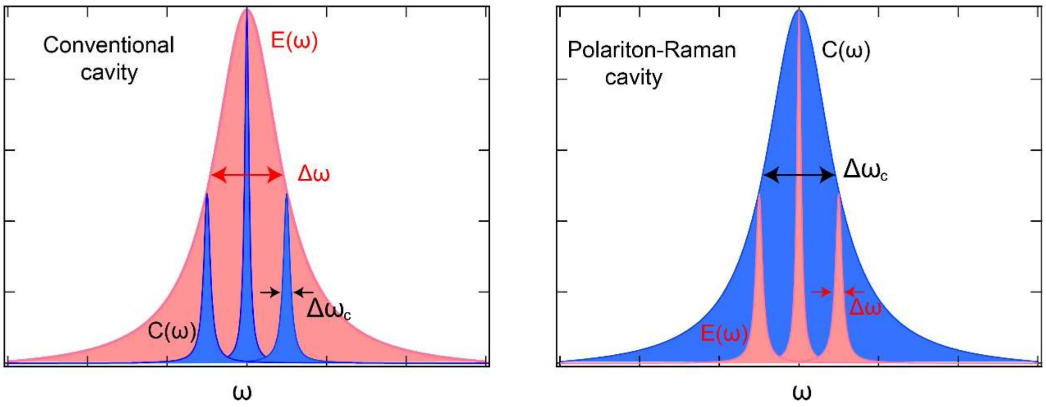


**Fig S9 |** Gain profile and cavity modes in a conventional laser (left) vs Polariton-Raman laser (right).

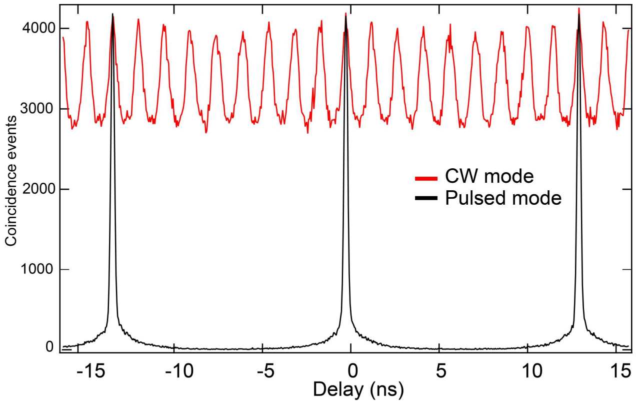


**Fig. S10** | Coincidence events recorded using HBT setup to measure second-order correlation, for the pump laser in CW mode (red) and picosecond pulsed mode (black).

## References


[1] A. K. Pattanayak, P. Das, A. Dhara, D. Chakrabarty, S. Paul, K. Gurnani, M. M. Brundavanam, and S. Dhara, A Steady-State Approach for Studying Valley Relaxation Using an Optical Vortex Beam, Nano Lett. **22**, 4712 (2022).

[2] D. Chakrabarty, A. Dhara, P. Das, K. Ghosh, A. R. Chaudhuri, and S. Dhara, *Anisotropic Exciton Polariton Pairs as a Platform for PT-Symmetric Non-Hermitian Physics*, arXiv:2305.17472.

[3] Y. Zhou et al., Stacking-Order-Driven Optical Properties and Carrier Dynamics in $ReS_2$, Adv. Mater. **32**, 1908311 (2020).

[4] A. Yariv, *Quantum Electronics*, 3rd ed (Wiley, New York, 1989).

[5] Y. Wu, X. Yang, and P. T. Leung, Theory of microcavity-enhanced Raman gain, Opt. Lett., OL **24**, 345 (1999).

[6] H. Yokoyama and S. D. Brorson, Rate equation analysis of microcavity lasers, Journal of Applied Physics **66**, 4801 (1989).

[7] X. Checoury, Z. Han, M. El Kurdi, and P. Boucaud, Deterministic measurement of the Purcell factor in microcavities through Raman emission, Phys. Rev. A **81**, 033832 (2010).

[8] G. Bjork and Y. Yamamoto, Analysis of semiconductor microcavity lasers using rate equations, IEEE J. Quantum Electron. **27**, 2386 (1991).

[9] B. Petrak, N. Djeu, and A. Muller, Purcell-enhanced Raman scattering from atmospheric gases in a high-finesse microcavity, Phys. Rev. A **89**, 023811 (2014).

[10] A. V. Kavokin, J. Baumberg, G. Malpuech, and F. P. Laussy, *Microcavities*, Second edition (Oxford University Press, Oxford, 2017).

[11] J. B. Khurgin and M. A. Noginov, How Do the Purcell Factor, the Q-Factor, and the Beta Factor Affect the Laser Threshold?, Laser & Photonics Reviews **15**, 2000250 (2021).
